# Supplementary material for: Asymptotically Fast Clebsch-Gordan Tensor Products with Vector Spherical Harmonics
Source: arXiv:2602.21466 source file (2026-02-25)
Supplement: Supplementary file 1 [file microbenchmarking.tex]

\section{Additional Benchmarks}
\label{sec:additional_benchmarks}

\begin{figure}[!htb]
\begin{tabular}{ccc}
  \includegraphics[height=0.16\textheight]{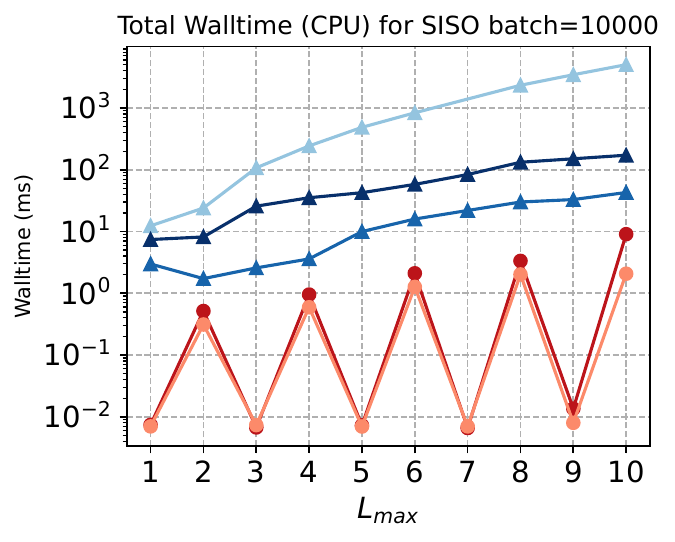} &   \includegraphics[height=0.16\textheight]{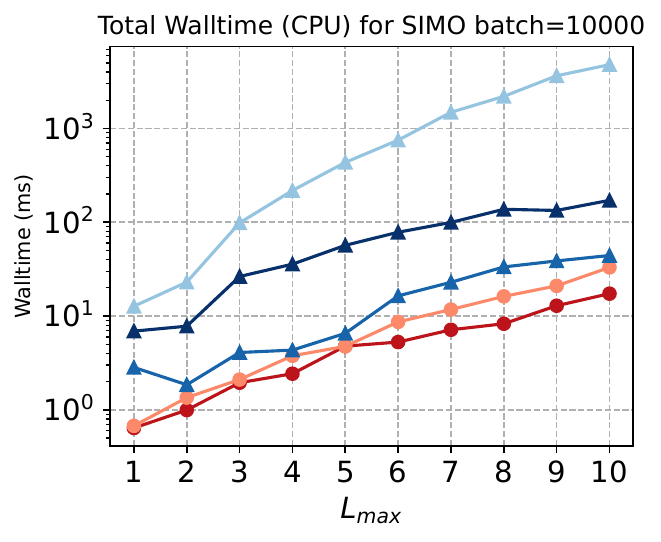} &  \includegraphics[height=0.16\textheight]{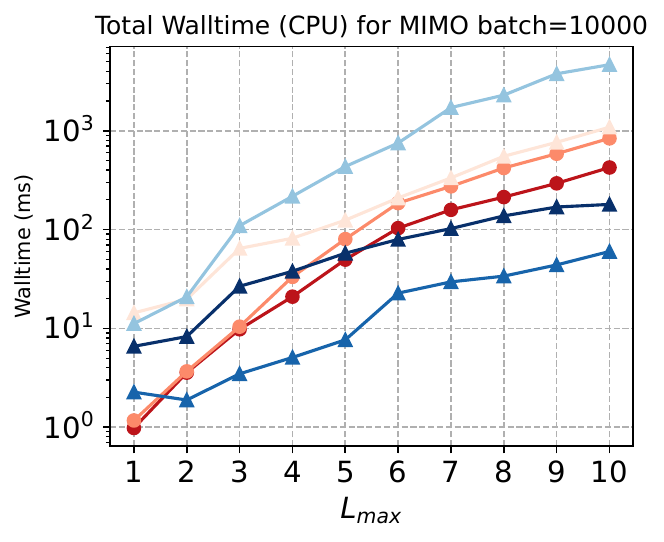} \\
  \includegraphics[height=0.16\textheight]{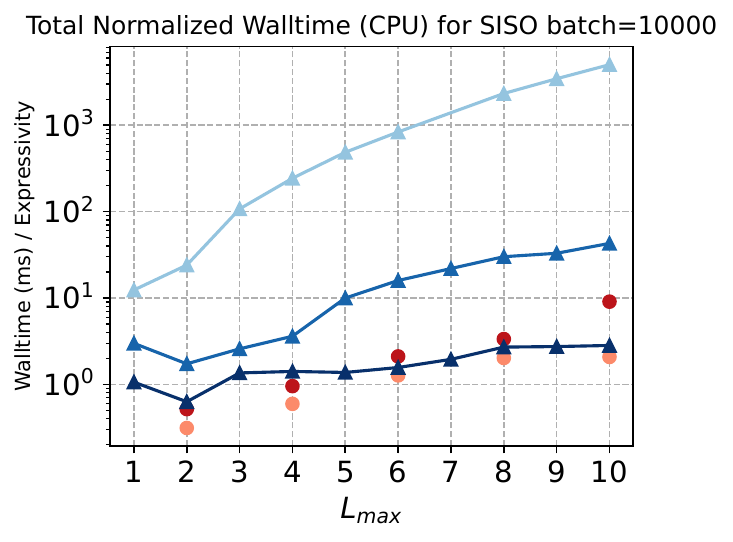} &   \includegraphics[height=0.16\textheight]{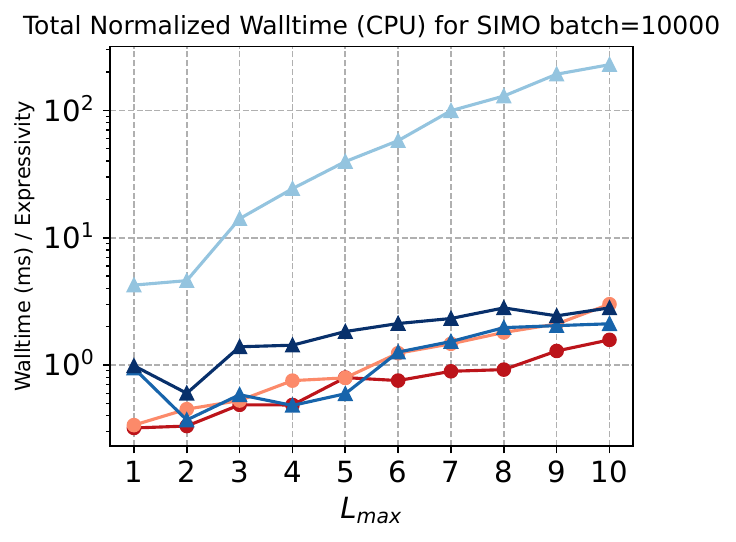} &  \includegraphics[height=0.16\textheight]{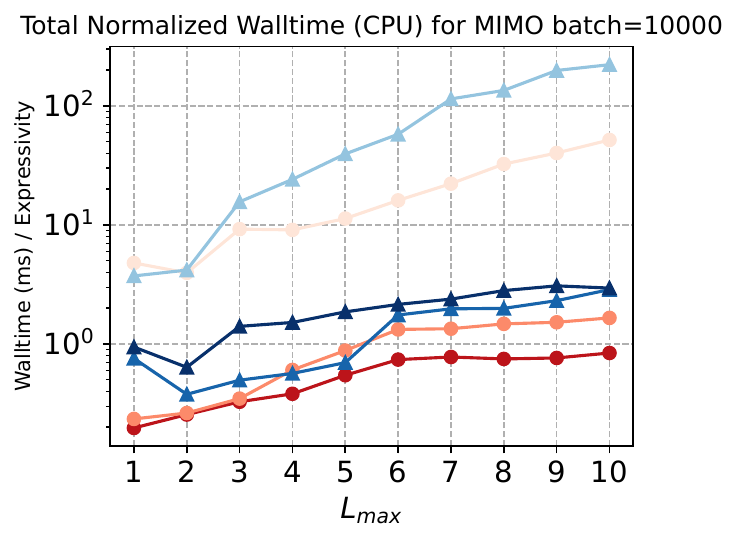} \\
  \includegraphics[height=0.16\textheight]{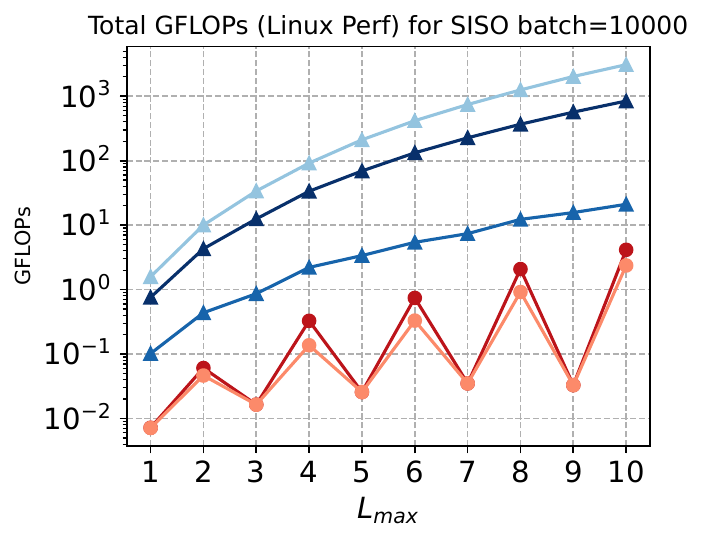} &   \includegraphics[height=0.16\textheight]{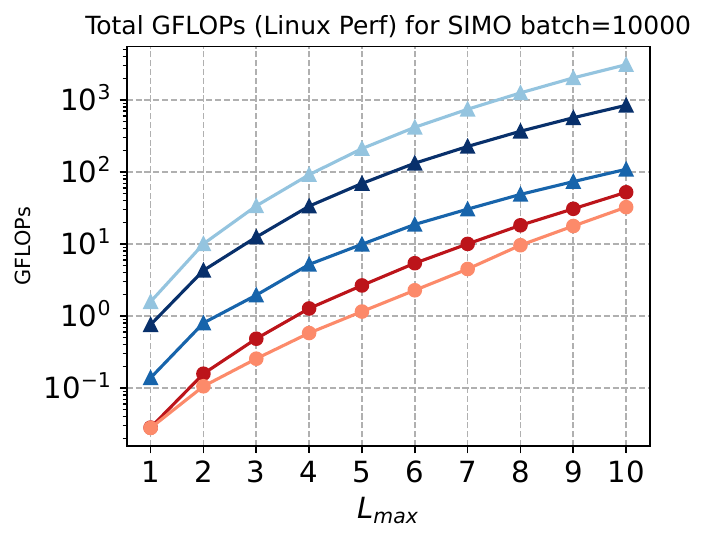} &  \includegraphics[height=0.16\textheight]{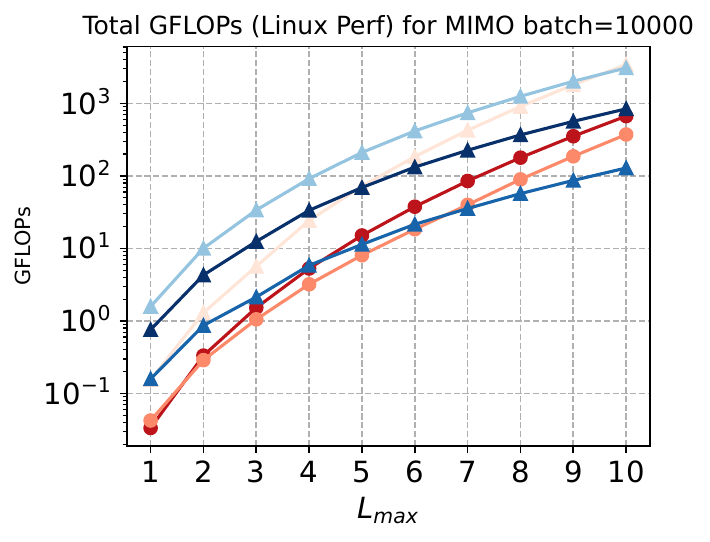} \\
  \includegraphics[height=0.16\textheight]{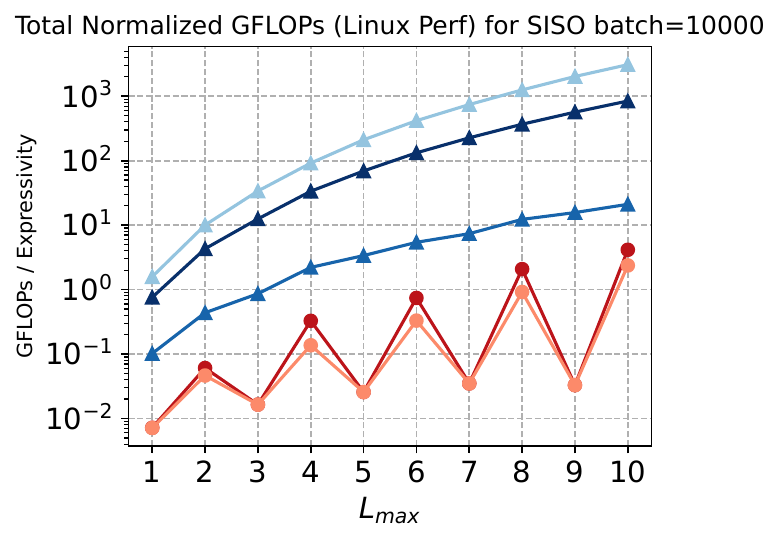} &   \includegraphics[height=0.16\textheight]{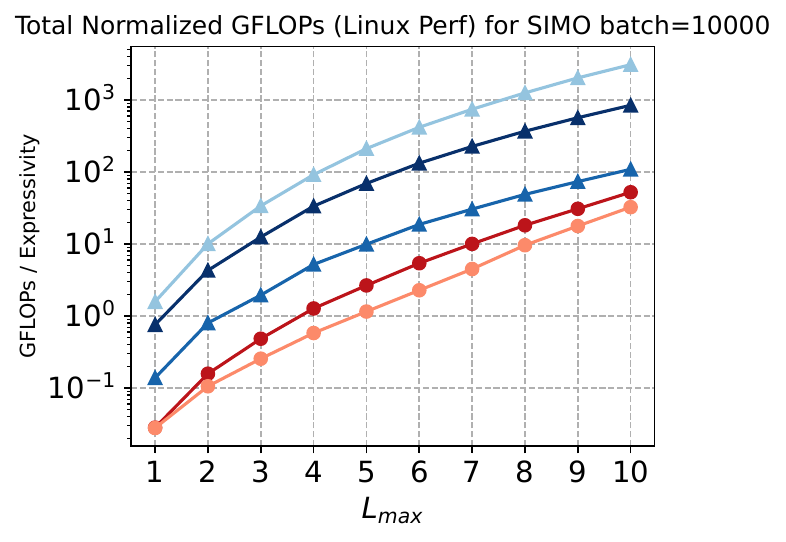} &  \includegraphics[height=0.16\textheight]{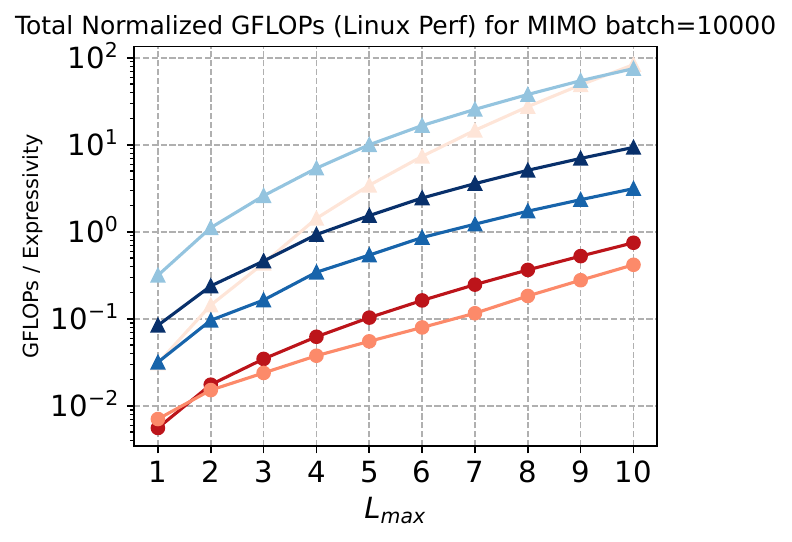} \\
\end{tabular}
\caption{Analysis of SISO, SIMO and MIMO performance for different tensor products on AMD EPYC 7313 : Total walltime (top row),  Total normalized walltime (second row), Total GFLOPs   (third row) and Total normalized GFLOPs (bottom row). Note that MTP only supports MIMO. We had to skip values due to profiling errors.}
\label{experiments:benchmarking_cpu}
\end{figure}

\begin{figure}[!htb]
\begin{tabular}{ccc}
  \includegraphics[height=0.16\textheight]{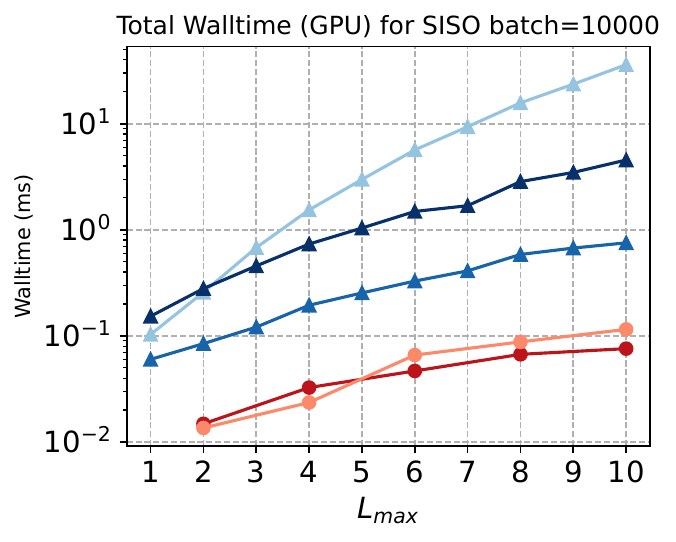} &   \includegraphics[height=0.16\textheight]{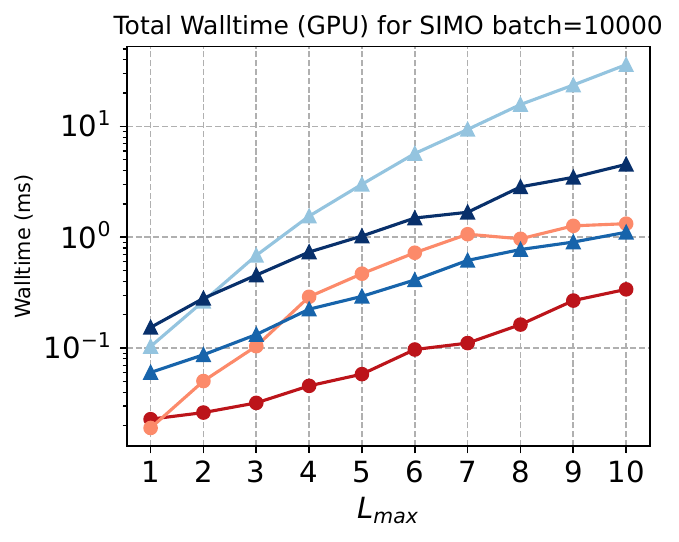} &  \includegraphics[height=0.16\textheight]{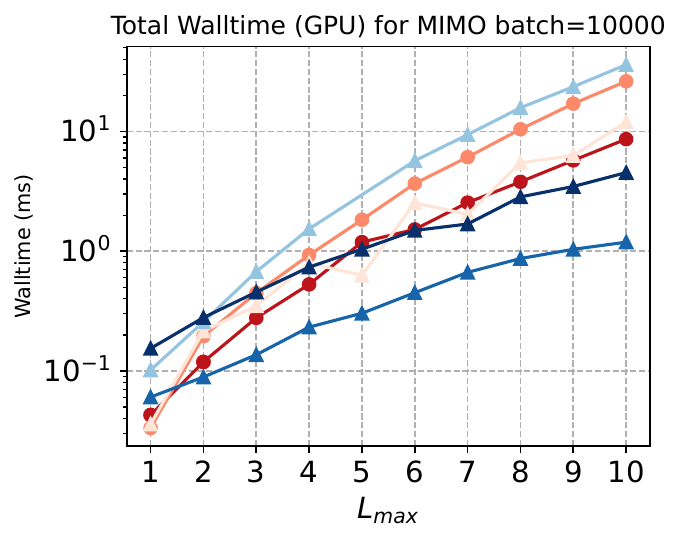} \\
  \includegraphics[height=0.16\textheight]{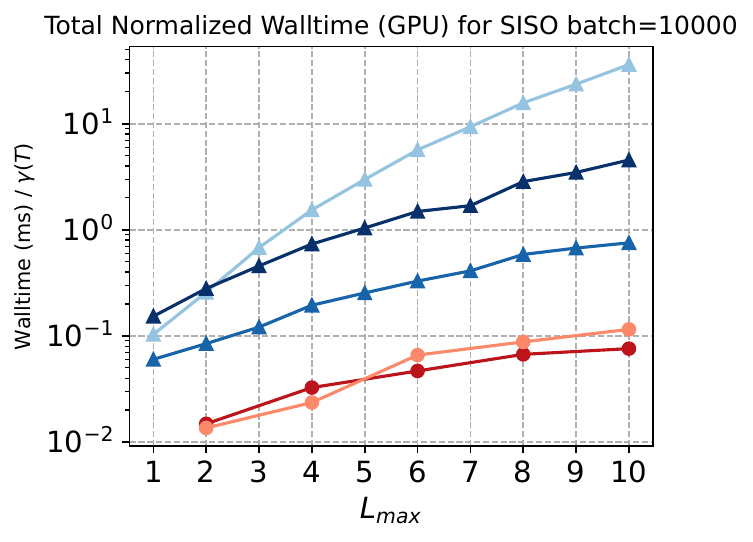} &   \includegraphics[height=0.16\textheight]{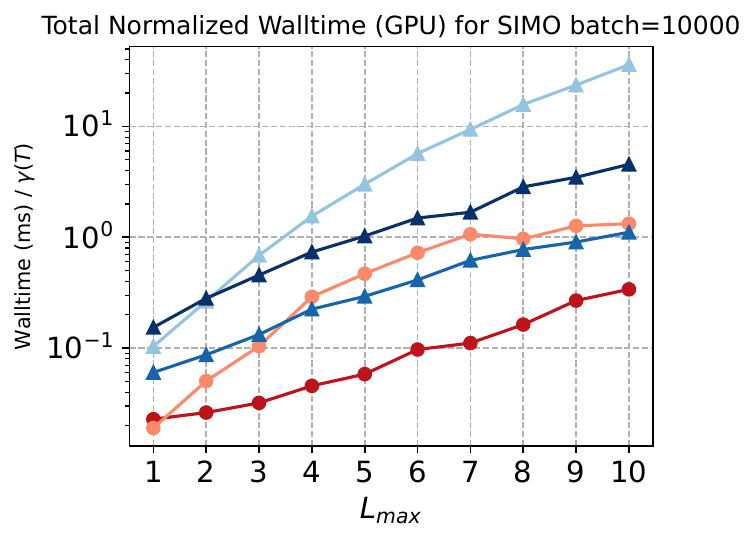} &  \includegraphics[height=0.16\textheight]{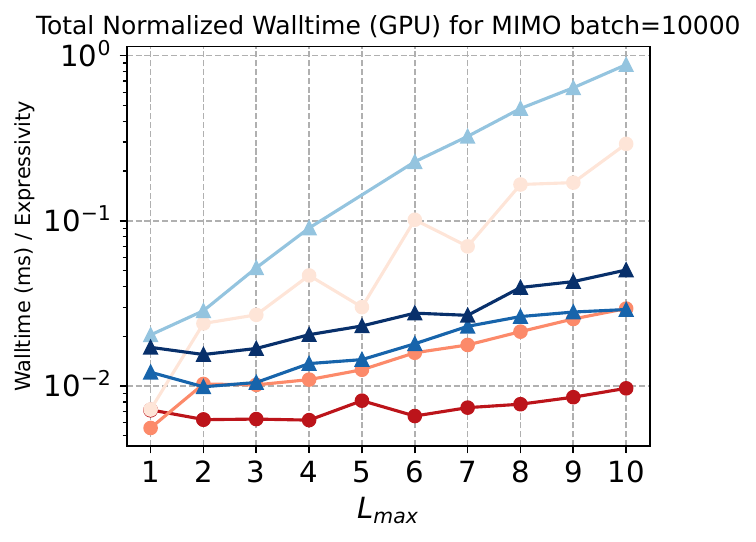} \\
  \includegraphics[height=0.16\textheight]{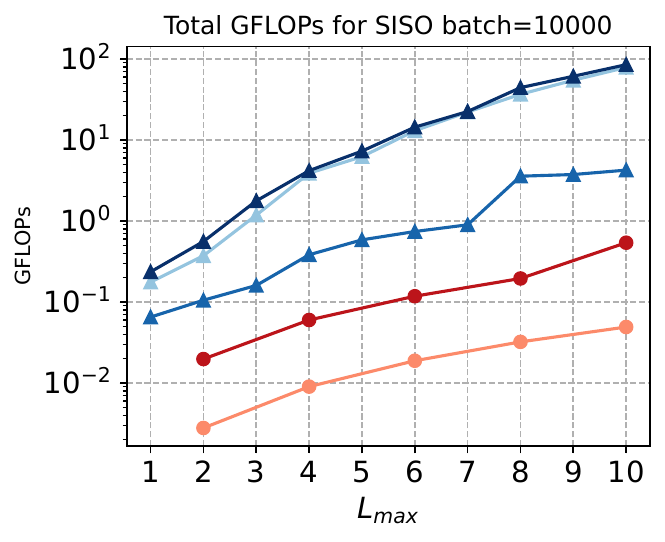} &   \includegraphics[height=0.16\textheight]{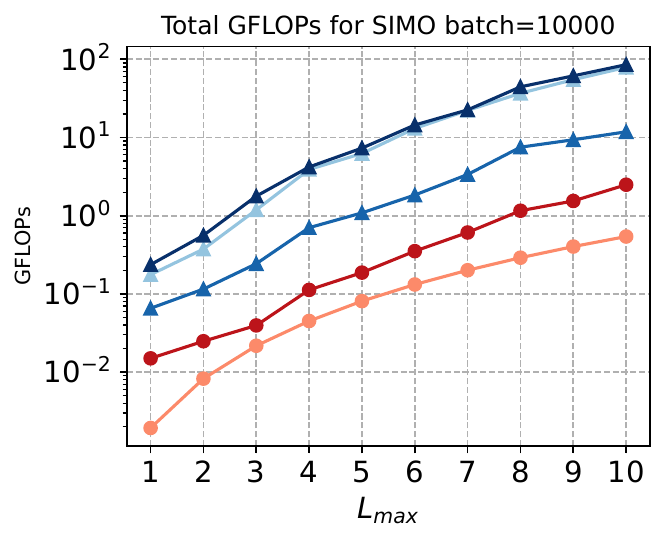} &  \includegraphics[height=0.16\textheight]{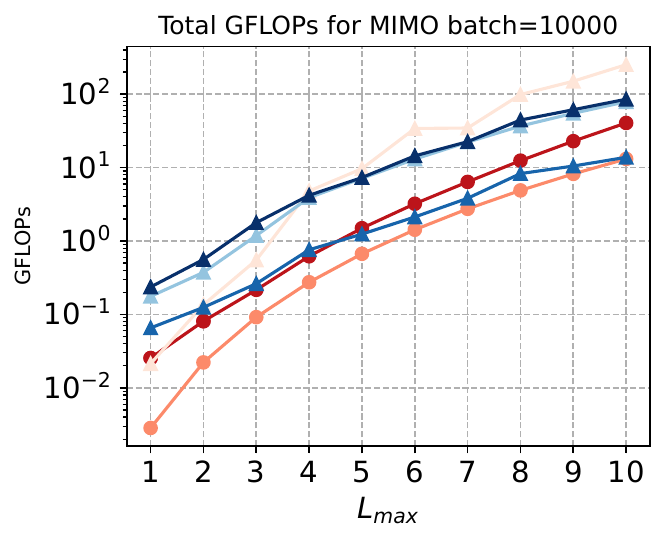} \\
  \includegraphics[height=0.16\textheight]{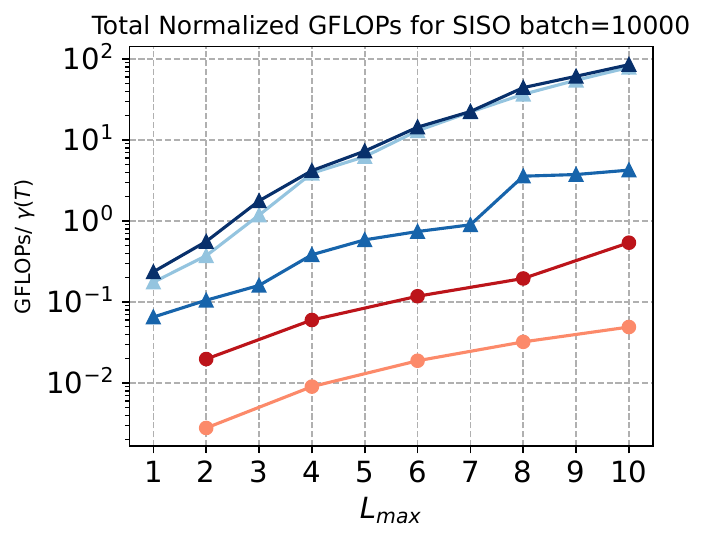} &   \includegraphics[height=0.16\textheight]{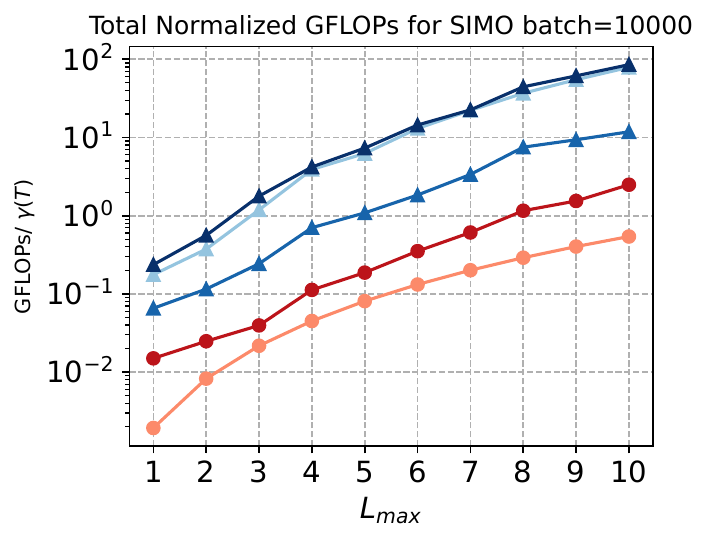} &  \includegraphics[height=0.16\textheight]{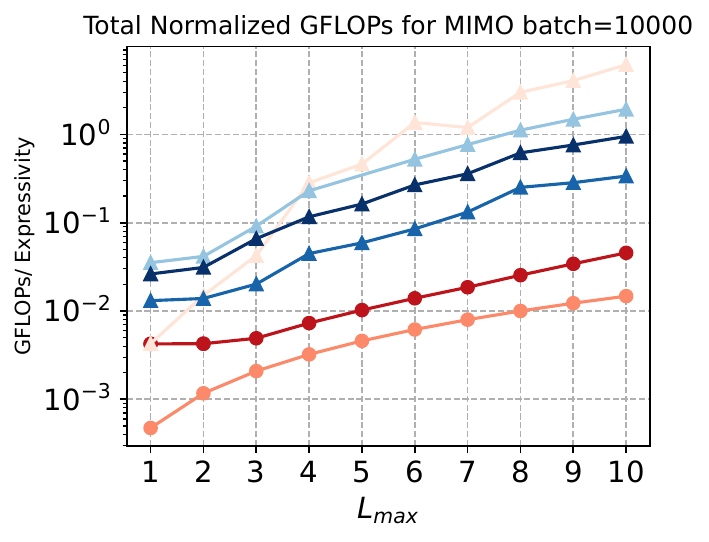} \\
  \includegraphics[height=0.16\textheight]
  {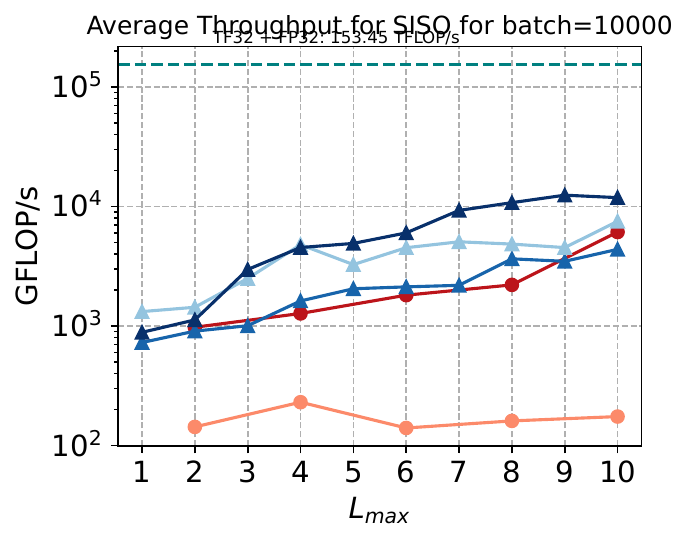} &   \includegraphics[height=0.16\textheight]{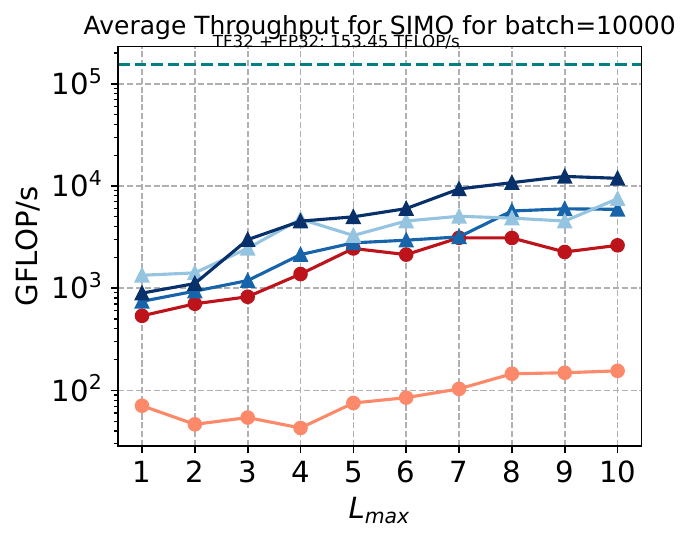} &  \includegraphics[height=0.16\textheight]{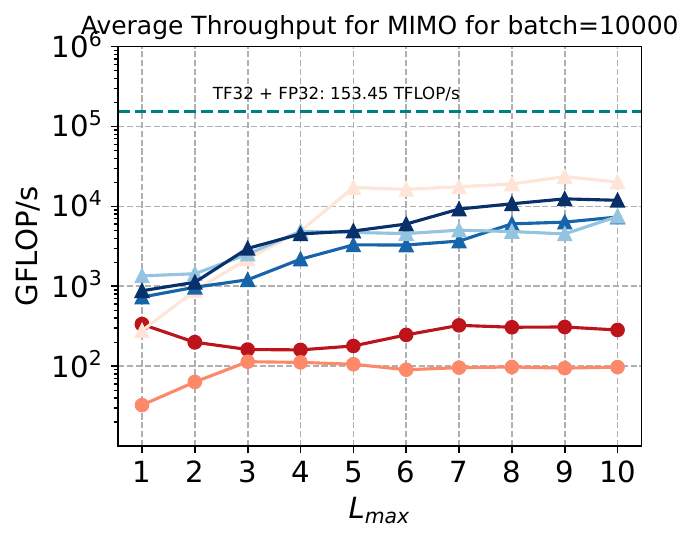} \\
\end{tabular}
\caption{Analysis of SISO, SIMO and MIMO performance for different tensor products on RTX A5500 : Total walltime (top row),  Total normalized walltime (second row), Total GFLOPs   (third row), Total normalized GFLOPs (fourth row) and Average throughput (bottom row). Note that MTP only supports MIMO. We had to skip values due to profiling errors.}
\label{experiments:benchmarking_gpu_rtx}
\end{figure}

\begin{figure}[!htb]
\begin{tabular}{ccc}
  \includegraphics[height=0.16\textheight]{figures/ICLR_experiments/walltime_gpu_SISO_10000.pdf} &   \includegraphics[height=0.16\textheight]{figures/ICLR_experiments/walltime_gpu_SIMO_10000.pdf} &  \includegraphics[height=0.16\textheight]{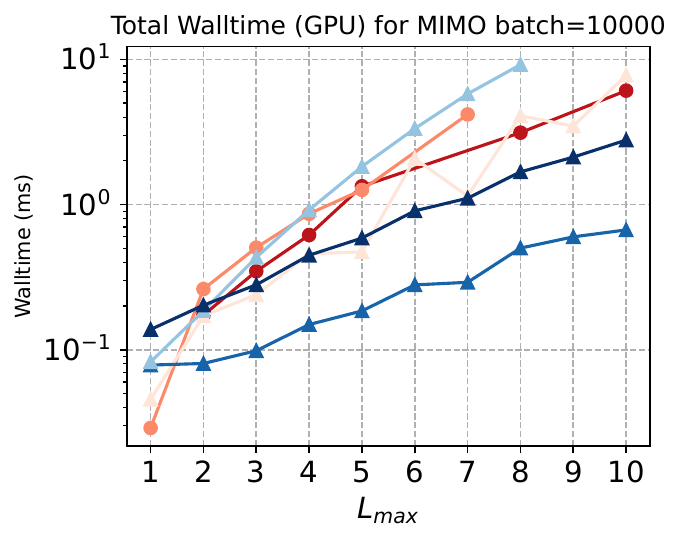} \\
  \includegraphics[height=0.16\textheight]{figures/ICLR_experiments/walltime_normalized_gpu_SISO_10000.pdf} &   \includegraphics[height=0.16\textheight]{figures/ICLR_experiments/walltime_normalized_gpu_SIMO_10000.pdf} &  \includegraphics[height=0.16\textheight]{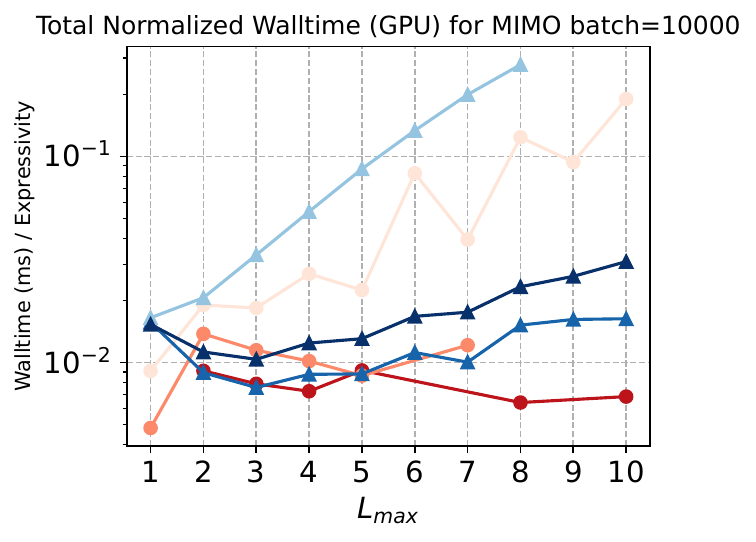} \\
  \includegraphics[height=0.16\textheight]{figures/ICLR_experiments/total_all_gflops_SISO_10000.pdf} &   \includegraphics[height=0.16\textheight]{figures/ICLR_experiments/total_all_gflops_SIMO_10000.pdf} &  \includegraphics[height=0.16\textheight]{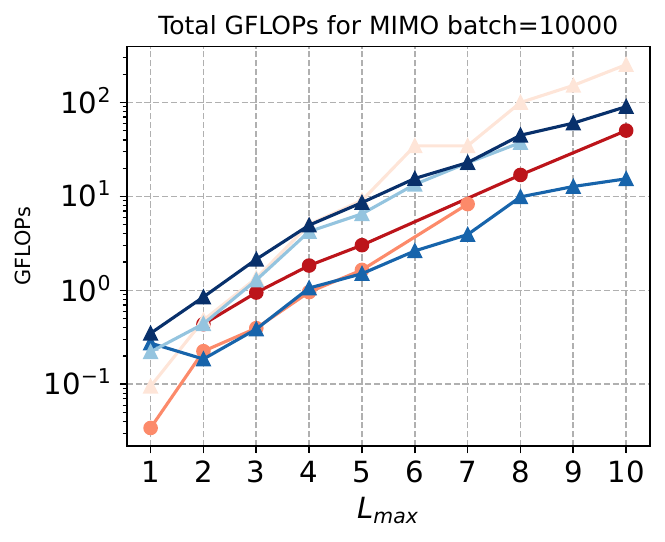} \\
  \includegraphics[height=0.16\textheight]{figures/ICLR_experiments/total_normalized_all_gflops_SISO_10000.pdf} &   \includegraphics[height=0.16\textheight]{figures/ICLR_experiments/total_normalized_all_gflops_SIMO_10000.pdf} &  \includegraphics[height=0.16\textheight]{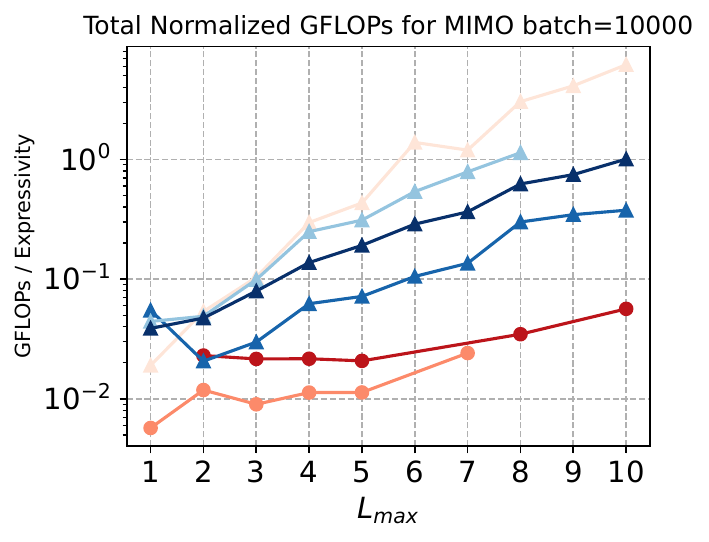} \\
  \includegraphics[height=0.16\textheight]
  {figures/ICLR_experiments/mean_all_gflops_SISO_10000.pdf} &   \includegraphics[height=0.16\textheight]{figures/ICLR_experiments/mean_all_gflops_SIMO_10000.pdf} &  \includegraphics[height=0.16\textheight]{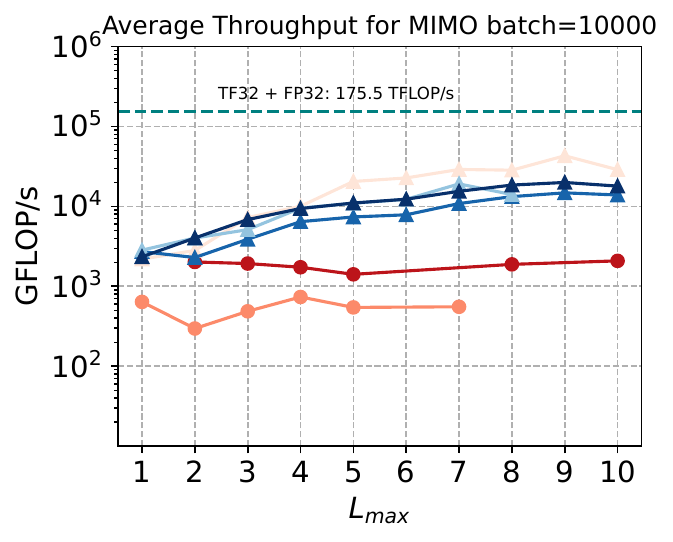} \\
\end{tabular}
\caption{Analysis of SISO, SIMO and MIMO performance for different tensor products on A100 : Total walltime (top row),  Total normalized walltime (second row), Total GFLOPs   (third row) and Total normalized GFLOPs (fourth row) and Average throughput (bottom row). Note that MTP only supports MIMO. We had to skip values due to profiling errors.}
\label{experiments:benchmarking_gpu_a100}
\end{figure}
